# Supplementary material for: Robust Execution of Contact-Rich Motion Plans by Hybrid Force-Velocity Control
Source: arXiv:1903.02715 source file (2019-03-07)
Supplement: Supplementary file 1 [file APPENDIX.tex]

% !TEX root = ../ICRA2019Hybrid.tex

\section*{APPENDIX}

Appendixes should appear before the acknowledgment.
